# Supplementary material for: ERGO: Event Relational Graph Transformer for Document-level Event Causality Identification
Source: arXiv:2204.07434 source file (2022-04-15)
Supplement: Supplementary file 1 [file 6_appendix.tex]

\appendix

\section{Dataset Statistics}
\label{app:dataset}
\paragraph{EventStoryLine} contains 22 topics, 258 documents, 5,334 events, 7,805 intra-sentence and 62,774 inter-sentence event pairs (1,770 and 3,885 of them are annotated with causal relations respectively). 
Following \citet{gao2019modeling}, we group documents according to their topics. Documents in the last two topics are used as the development data, and documents in the remaining 20 topics are employed for a 5-fold cross-validation.
\paragraph{Causal-TimeBank} contains 184 documents, 6,813 events, and 318 of 7,608 event pairs are annotated with causal relations.
Following \citep{liu2020knowledge} and \citep{phu2021graph}, we employ a 10-fold cross-validation evaluation. Note that the number of inter-sentence event pairs in Causal-TimeBank is quite small (i.e., only 18 pairs), following \citep{phu2021graph}, we only evaluate ECI performance for intra-sentence event pairs on Causal-TimeBank.

\section{Implementation Details}
\label{app:imp}
We implement our method based on Pytorch. We use uncased BERT-base \cite{devlin2018bert} or Longformser-base \citep{beltagy2020longformer} as the document encoder. For the BERT-base document encoder, we set the dynamic window size to 256, and divide documents into several overlapping windows with a step size 32. We optimize our model with AdamW \citep{loshchilov2017decoupled} using a learning rate of 0.00002 with a linear warm-up for the first 8\% steps. We apply dropout \citep{srivastava2014dropout} between layers and clip the gradients of model parameters to a max norm of 1.0. We perform early stopping based on the F1 score on the development set. We tune the hyper-parameters by grid search based on the development set performance: the number of layers $L \in$\{1, 2, 3\}, heads $C \in$\{1, 2, 4, 8\} for the relational graph transformer model, dropout rate $\in$ \{0.1, 0.2, 0.3\}, focusing parameter $\gamma \in$ \{0, 1, 2, 3\}, and weighting factor $\alpha$ of 0.75. 
The selected values from the tuning process include: 2 layers for $L$, 4 heads for $C$, 0.2 for the dropout rate, 2 for the focusing parameter $\gamma$.

\section{Results on the Development Data}

\begin{table}
    
    \centering
    \small
    \setlength{\tabcolsep}{8pt}
    \begin{tabular}{l|c|c|c}
    \toprule
         \textbf{Model}  & \textbf{Intra} & \textbf{Inter} &\textbf{Intra + Inter}  \\ \midrule
         ERGO$[\circ]$ &50.2 &30.3 &36.1  \\
         $\text{ERGO}_{1}[\circ]$ &47.8 &27.5 &34.6 \\
         $\text{ERGO}_{2}[\circ]$ &49.6 &28.9 &35.2  \\ 
         $\text{ERGO}_{3}[\circ]$ &46.7 &25.4 &33.3 \\
         \midrule
         ERGO$[\diamondsuit]$ &\textbf{55.6} &\textbf{34.1} &\textbf{38.9}  \\
       $\text{ERGO}_{1}[\diamondsuit]$ &51.1 &32.7 &35.3 \\
      $\text{ERGO}_{2}[\diamondsuit]$ &53.5 &33.0 &36.7  \\
      $\text{ERGO}_{3}[\diamondsuit]$ &50.6 &31.3 &34.1  \\
    \bottomrule
    \end{tabular}
       \caption{\label{app:tab:ablation}F1 Results of Ablation study on the development data of EventStoryLine, where $\text{ERGO}_{1}$ denotes ERGO w/ complete graph, $\text{ERGO}_{2}$ denotes ERGO w/o focal factor, $\text{ERGO}_{3}$ denotes ERGO w/ GCN.}
\end{table}

Table \ref{app:tab:ablation} shows the performance of models on the development data of EventStoryLine dataset. We can observe that all the components are still helpful for ERGO since eliminating either of them will harm the performance for both intra- and inter-sentence ECI.

\section{Comparison of the Number of Parameters}
As shown in Table~\ref{app:tab:comp}, we compare the number of parameters of our Relational Graph Transformer (RGT) with another two well-known Graph Neural Networks (GNNs): GCN and GAT \cite{velikovi2017graph}.
\begin{table}
    
    \centering
    \setlength{\tabcolsep}{7pt}
    \begin{tabular}{l|c}
    \toprule
         \textbf{Methods} & Number of Parameters\\\midrule
         GCN  &$\mathcal{O}(LD^{2})$\\
         GAT  &$\mathcal{O}(LHD^{2} + LD)$\\
         \midrule
         RGT (Ours) & $\mathcal{O}(LHD^{2})$\\
    \bottomrule
    \end{tabular}
    \caption{\label{app:tab:comp}
    Comparisons of the number of parameters between our RGT and two well-known GNNs (GCN and GAT). $L$ is the number of GNN layers, $H$ is the number of heads that GAT and RGT use, $D$ is the dimension of node features.
    }
\end{table}
